# Supplementary material for: The effect of competition and horizontal trait inheritance on invasion, fixation and polymorphism
Source: arXiv:1511.09062 source file (2015-11-29)
Supplement: Supplementary file 1 [file supplementarymaterials09112015.pdf]

# Supplementary materials to: The effect of horizontal trait inheritance on competitive exclusion and coexistence

Sylvain Billiard\*, Pierre Collet†, Régis Ferrière‡, Sylvie Méléard§, Viet Chi Tran¶

November 10, 2015

## Abstract

In these supplementary materials, we provide some details on the mathematical derivations of the results in Sections 3 and 4 of the main paper. Starting from a stochastic individual-based model, we provide approximations by solutions of ordinary differential equations or diffusion processes, depending on the chosen timescale. The properties of the system of ordinary differential equations and the fluctuations of the individual-based model around its limit are then studied.

In the main paper [1], an individual-based model in continuous time, with births, deaths, competition and horizontal transfers is introduced. The population is structured by a trait  $u \in \{A, a\}$ . The model is parameterized by  $K$ , the order of the initial population size. We denote by  $X_t^K$  and  $Y_t^K$  the densities of individuals with traits  $A$  and  $a$  at time  $t$ , so that the number of individuals with traits  $A$  and  $a$  are  $KX_t^K$  and  $KY_t^K$ . The parameter  $K$  also appears in the functions determining the dynamics of the process. An individual with trait  $u \in \{A, a\}$  reproduces at rate  $b_K(u)$ , dies at rate  $d_K(u) + KC_K(u, A)X_t^K + KC_K(u, a)Y_t^K$ . We denote by  $r_K(u) = b_K(u) - d_K(u)$  the natural growth rate of the population of trait  $u \in \{A, a\}$  in absence of competition. Individuals of trait  $u \in \{A, a\}$  transfer their trait to individuals of trait  $v \in \{A, a\}$  at a rate  $h_K(u, v, x, y)$  that can depend on the densities  $(x, y)$  of traits  $A$  and  $a$  in the population ( $u \neq v$ ). Several examples (namely FD, DD and BDA) of transfer rates are given in the main text.

We first recall the properties of the stochastic system. Several approximations in large population, when  $K \rightarrow +\infty$ , can be established. First, we will consider a deterministic limit, that solves a system of ordinary differential equations (ODE). We first show that there is no cycle. Then, the fixed points of this system and their stabilities are studied, which provides the phase

---

\*Univ. Lille, CNRS, UMR 8198 - Evo-Eco-Paleo, F-59000 Lille, France; E-mail: [sylvain.billiard@univ-lille1.fr](mailto:sylvain.billiard@univ-lille1.fr)

†CPHT, Ecole Polytechnique, CNRS, route de Saclay, 91128 Palaiseau Cedex-France; E-mail: [collet@cpht.polytechnique.fr](mailto:collet@cpht.polytechnique.fr)

‡Eco-Evolution Mathématique, CNRS UMR 7625, Ecole Normale Supérieure, 46 rue d'Ulm, 75230 Paris, France; E-mail: [ferriere@biologie.ens.fr](mailto:ferriere@biologie.ens.fr)

§CMAP, Ecole Polytechnique, CNRS, route de Saclay, 91128 Palaiseau Cedex-France; E-mail: [sylvie.meleard@polytechnique.edu](mailto:sylvie.meleard@polytechnique.edu)

¶Univ. Lille, CNRS, UMR 8524 - Laboratoire P. Painlevé, UFR de Mathématiques, F-59000 Lille, France; E-mail: [chi.tran@math.univ-lille1.fr](mailto:chi.tran@math.univ-lille1.fr)

diagrams displayed in Fig. 3.1 of the main paper. In the third section, the fluctuation process associated with the convergence of the individual-based model to the solutions of the ODE system is established. The fluctuations obtained for ‘quasi-critical’ populations on long timescales are also derived; we recover in the limit a diffusion process that is commented in the main paper.

## 1 Properties of the stochastic system

The generator of the stochastic birth-death process with competition and transfers is given in (2.1) of the paper [1]. Using Dynkin’s theorem with this generator and the test functions  $F(x, y) = x$  and  $F(x, y) = y$  allows to write the stochastic process  $(X^K, Y^K)$ , for fixed  $K$ , as

$$\begin{aligned} X_t^K &= X_0^K + \int_0^t P_K(X_s^K, Y_s^K) ds + M_t^{K,A}, \\ Y_t^K &= Y_0^K + \int_0^t Q_K(X_s^K, Y_s^K) ds + M_t^{K,a}, \end{aligned} \quad (1.1)$$

where  $M^{K,A}$  and  $M^{K,a}$  are local martingales and  $P_K$  and  $Q_K$  converge when  $K$  tends to infinity to  $P$  and  $Q$  defined as follows:

$$\begin{aligned} P(x, y) &= \left( r(A) - C(A, A)x - C(A, a)y + \frac{\alpha(A, a)}{\beta + \mu(x + y)} y \right) x \\ Q(x, y) &= \left( r(a) - C(a, A)x - C(a, a)y - \frac{\alpha(A, a)}{\beta + \mu(x + y)} x \right) y. \end{aligned} \quad (1.2)$$

Taking successively  $F(x, y) = x^2$ ,  $y^2$  and  $xy$  in (2.1) of the main paper, and comparing with Itô’s formula applied respectively to  $(X_t^K)^2$ ,  $(Y_t^K)^2$  and  $X_t^K Y_t^K$ , yields the quadratic variation of the martingales  $(M^{K,A}, M^{K,a})$ :

$$\begin{aligned} \langle M^{K,A} \rangle_t &= \frac{1}{K} \int_0^t b_K(A) X_s^K ds + \frac{1}{K} \int_0^t (d_K(A) + KC_K(A, A) X_s^K + KC_K(A, a) Y_s^K) X_s^K ds \\ &\quad + \frac{1}{K} \int_0^t K(h_K(A, a, X_s^K, Y_s^K) + h_K(a, A, X_s^K, Y_s^K)) X_s^K Y_s^K ds \\ \langle M^{K,a} \rangle_t &= \frac{1}{K} \int_0^t b_K(a) Y_s^K ds + \frac{1}{K} \int_0^t (d_K(a) + KC_K(a, A) X_s^K + KC_K(a, a) Y_s^K) Y_s^K ds \\ &\quad + \frac{1}{K} \int_0^t K(h_K(A, a, X_s^K, Y_s^K) + h_K(a, A, X_s^K, Y_s^K)) X_s^K Y_s^K ds \\ \langle M^{K,A}, M^{K,a} \rangle_t &= -\frac{1}{K} \int_0^t K(h_K(A, a, X_s^K, Y_s^K) + h_K(a, A, X_s^K, Y_s^K)) X_s^K Y_s^K ds. \end{aligned}$$

## 2 Convergence to the solution of a system of ODE

If the parameters satisfy

**Assumption 2.1**  $b_K(u) \rightarrow b(u)$ ,  $d_K(u) \rightarrow d(u)$ ,  $KC_K(u, v) \rightarrow C(u, v)$  and

$$\lim_{K \rightarrow \infty} Kh_K(A, a, x, y) = \frac{\tau(A, a)}{\beta + \mu(x + y)},$$

then, we can prove the following convergence.

**Proposition 2.2** *When  $K \rightarrow \infty$ , under Assumptions 2.1, and if  $(X_0^K, Y_0^K) \rightarrow (x_0, y_0)$ , the sequence of stochastic processes  $(X^K, Y^K)_{K \in \mathbb{N}^*}$  converges in probability to the unique solution  $(x, y)$  of the following system of ODE:*

$$\begin{aligned}\frac{dx}{dt} &= \left( r(A) - C(A, A)x - C(A, a)y + \frac{\alpha(A, a)}{\beta + \mu(x + y)} y \right) x \\ \frac{dy}{dt} &= \left( r(a) - C(a, A)x - C(a, a)y - \frac{\alpha(A, a)}{\beta + \mu(x + y)} x \right) y,\end{aligned}\tag{2.1}$$

with initial conditions  $(x_0, y_0)$ .

**Proof** One can easily prove that the martingale parts in (1.1) tend to 0. Therefore, the stochastic system  $(X^K, Y^K)$  converges uniformly on any time interval  $[0, T]$  to the solution of the dynamical system (2.1). Such result can be found in [4].  $\square$

### 3 Properties of the dynamical system (2.1)

The system (2.1) in the positive quadrant is of the form

$$\frac{dx}{dt} = P(x, y); \quad \frac{dy}{dt} = Q(x, y),\tag{3.1}$$

where the rational fractions  $P$  and  $Q$  have been defined in (1.2).

Expressing (2.1) in terms of the size of the population  $n_t = x_t + y_t$  and proportion of trait  $A$ ,  $p_t = x_t/n_t$ , we obtain:

$$\begin{aligned}\frac{dn}{dt} &= n \left( p r(A) + (1 - p) r(a) \right. \\ &\quad \left. - C(A, A) p^2 n - (C(A, a) + C(a, A)) p(1 - p)n - C(a, a) (1 - p)^2 n \right) \\ \frac{dp}{dt} &= p(1 - p) \left( r(A) - r(a) \right. \\ &\quad \left. + np(C(a, A) - C(A, A)) + n(1 - p)(C(a, a) - C(A, a)) + \alpha(A, a) \frac{n}{\beta + \mu n} \right).\end{aligned}\tag{3.2}$$

These equations are generalizations of the classical equation of population genetics with two alleles under selection [7], in which we have made the influence of demography explicit. Eq. (3.2) is useful to analyze the behavior of the system.

We first exclude the possibility of cycles contained in the positive quadrant.

**Proposition 3.1** *Assume that  $C(A, A) > 0$  and  $C(a, a) > 0$ . Then the function  $\varphi(x, y) = \frac{1}{xy}$  is a Dulac function in  $(\mathbb{R}_+^*)^2$ . As a consequence, the system (3.1) has no cycle in  $(\mathbb{R}_+^*)^2$ .*

**Proof** A Dulac function  $\varphi(x, y)$  in  $(\mathbb{R}_+^*)^2$  is a smooth non vanishing function such that

$$\partial_x(\varphi P) + \partial_y(\varphi Q)$$

has the same sign in the domain  $(\mathbb{R}_+^*)^2$ . A simple computation gives

$$\partial_x(\varphi P) + \partial_y(\varphi Q) = -\frac{C(A, A)x + C(a, a)y}{xy} < 0,$$

for  $(x, y) \in (\mathbb{R}_+^*)^2$ . The Bendixon-Dulac Theorem [3, 5] allows to conclude that there is no cycle in the domain.  $\square$

From this result and the Poincaré Birkhoff theorem [3, 5] we conclude that any accumulation point of any trajectory starting inside the positive quadrant is either a fixed point or is on the boundary. We now investigate the dynamics on the boundary of the positive quadrant which is an invariant set.

**Proposition 3.2** *We define*

$$\bar{x} = \frac{r(A)}{C(A, A)}; \bar{y} = \frac{r(a)}{C(a, a)}.$$

*The points  $(0, 0)$  and  $(0, \bar{y})$  and  $(\bar{x}, 0)$  are the only stationary points on the boundary. The origin is unstable and the two other points are stable for the dynamics on the boundary. Their transverse stability/instability is given by the sign of the fitness function:*

$$S(A, a) = r(A) - \frac{C(A, a)}{C(a, a)}r(a) + \frac{\alpha(A, a)r(a)}{\beta C(a, a) + \mu r(a)}. \quad (3.3)$$

The proof is left to the reader. This implies that any accumulation point of any trajectory starting inside the positive quadrant is a fixed point. We now investigate the fixed points inside the positive quadrant.

**Proposition 3.3** *Besides the fixed points in the boundary, there is*

- i) in the BDA case,  $\beta \neq 0; \mu \neq 0$ , there are at most 3 stationary points,*
  - ii) in the FD case ( $\beta = 0; \mu = 1$ ), there are at most 2 stationary points,*
  - iii) in the DD case ( $\beta = 1; \mu = 0$ ), there are at most 1 stationary point,*
- or a line of fixed points inside  $\mathbb{R}_+^2$ .*

**Proof** It is easier to consider the system in its form (3.2). The stationary points are denoted by  $(n, p)$  for convenience. They satisfy

$$\begin{aligned} 0 &= n \left( p r(A) + (1 - p) r(a) \right. \\ &\quad \left. - C(A, A) p^2 n - (C(A, a) + C(a, A)) p(1 - p)n - C(a, a) (1 - p)^2 n \right) \\ 0 &= p(1 - p) \left( r(A) - r(a) \right. \\ &\quad \left. + np(C(a, A) - C(A, A)) + n(1 - p)(C(a, a) - C(A, a)) + \alpha(A, a) \frac{n}{\beta + \mu n} \right). \end{aligned}$$

If  $n \neq 0$  and  $p \notin \{0, 1\}$ , we deduce from the first equation that

$$n = \frac{pr(A) + (1-p)r(a)}{Q(p)}$$

where

$$Q(p) = C(A, A)p^2 + (C(A, a) + C(a, A))p(1-p) + C(a, a)(1-p)^2 \neq 0$$

for  $p \in (0, 1)$ . Replacing  $n$  by this quantity, we write the second equation as

$$\begin{aligned} 0 = & \frac{p(1-p)}{Q(p)(\beta Q(p) + \mu(pr(A) + (1-p)r(a)))} \times \\ & \left( (r(A) - r(a))Q(p)(\beta Q(p) + \mu(pr(A) + (1-p)r(a))) \right. \\ & + (pr(A) + (1-p)r(a))(\beta Q(p) + \mu(pr(A) + (1-p)r(a))) \\ & (p(C(a, A) - C(A, A)) + (1-p)(C(a, a) - C(A, a))) \\ & \left. + \alpha(A, a)(pr(A) + (1-p)r(a))Q(p) \right). \end{aligned}$$

When  $\beta \neq 0$  and  $\mu \neq 0$  (BDA case), the term between the large brackets is a priori a polynomial in  $p$  of degree 4. But explicit computation shows that the term of order 4 vanishes. Then this polynomial is of degree 3 and there are at most 3 stationary points inside the domain. In FD cases, the expression simplifies as  $\frac{p(1-p)}{Q(p)}$  times a polynomial of degree 2 and there are at most two stationary points. The DD case reduces to a Lotka-Volterra system.  $\square$

To obtain more insight on the limiting dynamics, we use the Poincaré index (see [3, 5]).

Let us first remark that the trace of the Jacobian matrix of any fixed point  $(x_0, y_0)$  inside  $\mathbb{R}_+^2$ , is equal to

$$-C(A, A)x_0 - C(a, a)y_0 < 0.$$

This implies that any fixed point inside the positive quadrant is either a sink (index 1), a saddle (index  $-1$ ) or a non-hyperbolic point of index 0 with a negative eigenvalue of the Jacobian matrix (because the vector field is analytic, see [3]). We use the circuit drawn in the following picture with anticlockwise orientation. The largest radius is chosen large enough such that there are no fixed points outside the loop. The fixed points  $(\bar{x}, 0)$  and  $(0, \bar{y})$  on the boundaries are denoted by  $A$  and  $a$  on the picture, with an abuse of notation.

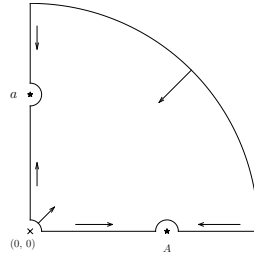

The arrows represent the directions of the vector field along the different part of the circuit. Note that the arrow on the largest arc is only for FD or BDA cases. It can be shown in all cases that for a radius large enough, the large arc contributes  $1/4$  to the index.

**Proposition 3.4** *Assume all fixed points are hyperbolic. The only possibilities are as follows:*

- *if  $A$  and  $a$  are unstable points, the index of the circuit is 1 and there is either one stable point inside the domain or 3 fixed points: 2 stable nodes and one saddle point.*
- *if  $A$  and  $a$  are stable points, the index is -1 and there is either one saddle point inside or 3 fixed points: 2 saddle points and one stable point.*
- *if one of the points  $A$  or  $a$  is an unstable node and the other one a saddle point, then the index is 0 and we have either 0 fixed point or two fixed points: one saddle point and one stable point.*

This proposition follows from the Poincaré-Hopf theorem: the index of the curve is equal to the sum of the indices of the fixed points inside the domain (see [3, 5]). Combining this result with Proposition 3.2, one can decide between the different possibilities depending on the parameters.

The diagrams in Figure 3.1 (of the main paper) realize the different situations described above. However, there may exist other diagrams in accordance with Proposition 3.4 that we have never observed numerically. We are yet unable to prove or disprove the existence of such other diagrams. In the case of non hyperbolic fixed points inside the positive quadrant (with index 0 as mentioned previously), an analogue of Proposition 3.4 can be established. This situation is however exceptional since it implies a nonlinear (polynomial) relation between the coefficients.

In the case of nearly close phenotypic effects (cf. Special case 2 in Section 3 of the main paper), we use the same technique as in [2]. For  $\varepsilon = 0$  (equal coefficients), the system has a line of fixed points which is globally transversally stable. By the stability of normally hyperbolic invariant sets (see [6]), we deduce using Proposition 3.4 that the only possible phase diagrams are those of Figure 3.1 of the main paper, or a stable line of fixed points.

We can use perturbation theory in  $\varepsilon$  to investigate this situation. The bifurcation hypersurfaces separating in the parameter space the domains of different phase diagrams, can be computed at all orders of  $\varepsilon$ . We can then deduce the volume of these domains. Choosing the parameters uniformly at random in a ball of radius  $\varepsilon$  around the neutral case provides the probabilities of the various phase diagrams that are mentioned in Section 3-Special case 2 of the main paper.

## 4 Fluctuations of the individual-based model around the solution of (2.1)

Now, let us study the fluctuations of  $(X^K, Y^K)$  around its limit, i.e. the solution  $(x, y)$  of (2.1). We introduce the sequence  $(\eta_t^{K,A}, \eta_t^{K,a}) = (\sqrt{K}(X_t^K - x, Y_t^K - y))_{K \in \mathbb{N}^*}$ . We get

$$\begin{aligned}\eta_t^{K,A} &= \sqrt{K}(X_0^K - x_0) + \int_0^t \sqrt{K}(P_K(X_s^K, Y_s^K) - P(x, y))ds + \sqrt{K}M_t^{K,A}, \\ \eta_t^{K,a} &= \sqrt{K}(Y_0^K - y_0) + \int_0^t \sqrt{K}(Q_K(X_s^K, Y_s^K) - Q(x, y))ds + \sqrt{K}M_t^{K,a}.\end{aligned}$$

We remark that the limiting martingale parts do not disappear anymore. Assume that we can write  $h_K(u, v, x, y) = \tau_K(u, v)/(\beta + \mu(x + y))$ , and let us introduce the notation  $\alpha_K(u, v) = \tau_K(u, v) - \tau_K(v, u)$  and  $\alpha(u, v) = \tau(u, v) - \tau(v, u)$ .

**Proposition 4.1** *Suppose that the demographic and transfer rates satisfy Assumptions 2.1 with*

$$\lim_{K \rightarrow +\infty} \sqrt{K}(r_K(u) - r(u)) = 0 \text{ for } u \in \{A, a\} \text{ and } \lim_{K \rightarrow +\infty} \sqrt{K}(\alpha_K(A, a) - \alpha(A, a)) = 0.$$

*Assume moreover that the sequence  $(\eta_0^{K,A}, \eta_0^{K,a})$  converges in law to  $(\eta_0^A, \eta_0^a)$ .*

*Then, the sequence of processes  $(\eta_t^{K,A}, \eta_t^{K,a})_{K \in \mathbb{N}^*}$  converges in law to the unique (continuous) solution of following diffusion*

$$\begin{pmatrix} \eta_t^A \\ \eta_t^a \end{pmatrix} = \begin{pmatrix} \eta_0^A \\ \eta_0^a \end{pmatrix} + \begin{pmatrix} M_t^A \\ M_t^a \end{pmatrix} + \int_0^t J(x_s, y_s) \begin{pmatrix} \eta_s^A \\ \eta_s^a \end{pmatrix} ds \quad (4.1)$$

where  $J(x_s, y_s)$  is the following matrix:

$$J(x, y) = \begin{pmatrix} J_{11}(x, y) & J_{12}(x, y) \\ J_{21}(x, y) & J_{22}(x, y) \end{pmatrix}$$

with:

$$\begin{aligned} J_{11}(x, y) &= r(A) - 2C(A, A)x - C(A, a)y + \alpha(A, a) \frac{\beta y + \mu y^2}{(\beta + \mu(x + y))^2} \\ J_{12}(x, y) &= -C(A, a)x + \alpha(A, a) \frac{\beta x + \mu x^2}{(\beta + \mu(x + y))^2} \\ J_{21}(x, y) &= -C(a, A)y + \alpha(a, A) \frac{\beta y + \mu y^2}{(\beta + \mu(x + y))^2} \\ J_{22}(x, y) &= r(a) - 2C(a, a)y - C(a, A)x + \alpha(a, A) \frac{\beta x + \mu x^2}{(\beta + \mu(x + y))^2}. \end{aligned}$$

$(M_t^A, M_t^a)_{t \geq 0}$  is a continuous square integrable martingale started at 0 with previsible quadratic variation:

$$\begin{aligned} \langle M^A \rangle_t &= \int_0^t \left[ (b(A) + (d(A) + C(A, A)x_s + C(A, a)y_s))x_s + (\tau(A, a) + \tau(a, A)) \frac{x_s y_s}{\beta + \mu(x_s + y_s)} \right] ds \\ \langle M^a \rangle_t &= \int_0^t \left[ (b(a) + (d(a) + C(a, A)x_s + C(a, a)y_s))y_s + (\tau(A, a) + \tau(a, A)) \frac{x_s y_s}{\beta + \mu(x_s + y_s)} \right] ds \\ \langle M^A, M^a \rangle_t &= - \int_0^t (\tau(A, a) + \tau(a, A)) \frac{x_s y_s}{\beta + \mu(x_s + y_s)} ds. \end{aligned}$$

**Proof** We start with the computation of the SDE satisfied by  $\eta_t^{K,A}$ . By substracting (2.1) to

(1.1), we obtain:

$$\begin{aligned}
\eta_t^{K,A} = & \sqrt{K}(X_0^K - x_0) + \sqrt{K} M_t^{K,A} + \int_0^t (r_K(A) - C(A, A)X_s^K - C(A, a)Y_s^K) \eta_s^{K,A} ds \\
& + \int_0^t \sqrt{K}(r_K(A) - r(A))x_s ds - \int_0^t (C(A, A)\eta_s^{K,A} + C(A, a)\eta_s^{K,a})x_s ds \\
& + \int_0^t \left[ \alpha(A, a) \frac{\beta(\eta_s^{K,A}Y_s^K + x_s\eta_s^{K,a}) + \mu(\eta_s^{K,a}x_sX_s^K + \eta_s^{K,A}y_sY_s^K)}{(\beta + \mu(X_s^K + Y_s^K))(\beta + \mu(x_s + y_s))} \right] ds \\
& + \int_0^t \left[ \sqrt{K}(\alpha_K(A, a) - \alpha(A, a)) \frac{Y_s^K X_s^K}{\beta + \mu(X_s^K + Y_s^K)} \right] ds
\end{aligned}$$

where  $M_t^{K,A}$  is the martingale introduced in (1.1). Making  $K$  tend to infinity in the previous equation and in the expressions of the quadratic variations of the martingale parts gives the first coordinate of (4.1). We proceed similarly for the second coordinate.  $\square$

## 5 Diffusion limit for ‘quasi-critical’ populations in accelerated time

Let us now consider the diffusion-approximation scalings introduced in Subsection 4.2 of the main paper [1].

**Proposition 5.1** *Assume that  $b_K(u) = \gamma(u) + \frac{\nu(u)}{K}$  and  $d_K(u) = \gamma(u) + \frac{\rho(u)}{K}$ ,  $C_K(u, v) = \frac{C(u, v)}{K}$  and  $Kh_K(u, v, x, y) = \frac{\zeta + \frac{1}{K}\theta(u, v)}{\beta + \mu(x + y)}$ . Then, if  $(X_0^K, Y_0^K)$  converges in law to  $(x_0, y_0)$ , then the process  $((X_{Kt}^K, Y_{Kt}^K), t \in [0, T])$  converges to the solution of the stochastic differential system when  $K \rightarrow +\infty$ :*

$$\begin{aligned}
\bar{X}_t = & x_0 + \int_0^t \left[ (\nu(A) - \rho(A) - C(A, A)\bar{X}_s - C(A, a)\bar{Y}_s)\bar{X}_s + \frac{\theta(A, a) - \theta(a, A)}{\beta + \mu(\bar{X}_s + \bar{Y}_s)}\bar{X}_s\bar{Y}_s \right] ds \\
& + \int_0^t \sqrt{2\gamma(A)\bar{X}_s} dB_s^A + \int_0^t \sqrt{\frac{2\zeta\bar{X}_s\bar{Y}_s}{\beta + \mu(\bar{X}_s + \bar{Y}_s)}} dB_s^h, \\
\bar{Y}_t = & y_0 + \int_0^t \left[ (\nu(a) - \rho(a) - C(a, A)\bar{X}_s - C(a, a)\bar{Y}_s)\bar{Y}_s - \frac{\theta(A, a) - \theta(a, A)}{\beta + \mu(\bar{X}_s + \bar{Y}_s)}\bar{X}_s\bar{Y}_s \right] ds \\
& + \int_0^t \sqrt{2\gamma(a)\bar{Y}_s} dB_s^a - \int_0^t \sqrt{\frac{2\zeta\bar{X}_s\bar{Y}_s}{\beta + \mu(\bar{X}_s + \bar{Y}_s)}} dB_s^h,
\end{aligned} \tag{5.1}$$

where  $B^A$ ,  $B^a$  and  $B^h$  are independent Brownian motions.

**Proof** Considering the process at the time scale  $Kt$  consists in multiplying all demographic parameters by  $K$ . At this time scale, the parameters have been chosen such that their contributions of order  $K$  vanishes in (1.1). Therefore straightforward computation in (1.1) and in the

expressions of the quadratic variations of the martingale parts yields the result. Indeed,

$$\begin{aligned}
X_{Kt}^K &= X_0^K + \int_0^t \left[ (\nu(A) - \rho(A) - C(A, A)X_s^K - C(A, a)Y_s^K)X_s^K \right. \\
&\quad \left. + \frac{\theta(A, a) - \theta(a, A)}{\beta + \mu(X_s^K + Y_s^K)} X_s^K Y_s^K \right] ds + M_{Kt}^{K,a}, \\
Y_{Kt}^K &= Y_0^K + \int_0^t \left[ (\nu(a) - \rho(a) - C(a, A)X_s^K - C(a, a)Y_s^K)Y_s^K \right. \\
&\quad \left. - \frac{\theta(A, a) - \theta(a, A)}{\beta + \mu(X_s^K + Y_s^K)} X_s^K Y_s^K \right] ds + M_{Kt}^{K,a},
\end{aligned}$$

and

$$\begin{aligned}
\langle M^{K,A} \rangle_{Kt} &= \int_0^t \left( \gamma(A) + \frac{\nu(A)}{K} \right) X_s^K ds \\
&\quad + \int_0^t \left( \gamma(A) + \frac{\rho(A) + C(A, A)X_s^K + C(A, a)Y_s^K}{K} \right) X_s^K ds \\
&\quad + \int_0^t \frac{2\zeta + \frac{1}{K}\theta(A, a) + \frac{1}{K}\theta(a, A)}{\beta + \mu(X_s^K + Y_s^K)} X_s^K Y_s^K ds \\
\langle M^{K,a} \rangle_{Kt} &= \int_0^t \left( \gamma(a) + \frac{\nu(a)}{K} \right) Y_s^K ds \\
&\quad + \int_0^t \left( \gamma(a) + \frac{\rho(a) + C(a, A)X_s^K + C(a, a)Y_s^K}{K} \right) Y_s^K ds \\
&\quad + \int_0^t \frac{2\zeta + \frac{1}{K}\theta(A, a) + \frac{1}{K}\theta(a, A)}{\beta + \mu(X_s^K + Y_s^K)} X_s^K Y_s^K ds \\
\langle M^{K,A}, M^{K,a} \rangle_{Kt} &= - \int_0^t \frac{2\zeta + \frac{1}{K}\theta(A, a) + \frac{1}{K}\theta(a, A)}{\beta + \mu(X_s^K + Y_s^K)} X_s^K Y_s^K ds.
\end{aligned}$$

Making  $K$  tend to infinity gives the system (4.2) of the main paper, the Brownian parts being obtained by the representation theorem.  $\square$

**Acknowledgements:** S.B., S.M. and V.C.T. have been supported by the ANR MANEGE (ANR-09-BLAN-0215), the Chair “Modélisation Mathématique et Biodiversité” of Veolia Environnement-Ecole Polytechnique-Museum National d’Histoire Naturelle-Fondation X. V.C.T. also acknowledges support from Labex CEMPI (ANR-11-LABX-0007-01). R.F. acknowledges support from the Pépinière Interdisciplinaire CNRS-PSL “Eco-Evo-Devo” and the Partner University Fund.

## References

- [1] S. Billiard, P. Collet, R. Ferrière, S. Méléard, and V.C. Tran. The effect of horizontal trait inheritance on competitive exclusion and coexistence. Main paper, 2015.
- [2] P. Collet, S. Méléard, and J.A.J. Metz. A rigorous model study of the adaptive dynamics of Mendelian diploids. *Journal of Mathematical Biology*, page in press, 2012. (published online 21 July 2012).
- [3] F. Dumortier, J. Libre and J. Artés. Qualitative theory of planar differential systems. *Springer*, 2006.
- [4] S.N. Ethier and T.G. Kurtz. Markov Processes: Characterization and Convergence. *Wiley*, 2005.

- [5] Guckenheimer, J., Holmes P. *Nonlinear Oscillations, Dynamical Systems and Bifurcation of Vector Fields*. Springer (1983).
- [6] Hirsh, M., Pugh, C., Shub, M.: *Invariant Manifolds*. Lecture notes in Mathematics **583**. Springer-Verlag (1977).
- [7] J.A. Roughgarden. *Theory of population genetics and evolutionary ecology: an introduction*. 1971.
